# Supplementary material for: On Optimal Sampling for Learning SDF Using MLPs Equipped with Positional Encoding
Source: arXiv:2401.01391 source file (2024-12-22)
Supplement: Supplementary file 1 [file appendix.tex]

\documentclass[lettersize,journal]{IEEEtran}

\usepackage{epsfig}
\usepackage{graphicx}
\usepackage{amsmath}
\usepackage{amssymb}
\usepackage[citecolor=blue, colorlinks]{hyperref}
\usepackage{comment}
\usepackage{color}
\usepackage{overpic}
\usepackage{subcaption}
\usepackage[dvipsnames]{xcolor}
\usepackage[switch,columnwise]{lineno}
\runningpagewiselinenumbers
\linenumbers

\DeclareMathOperator*{\argmax}{arg\,max}
\DeclareMathOperator*{\argmin}{arg\,min}

\hyphenation{op-tical net-works semi-conduc-tor IEEE-Xplore}
\def\BibTeX{{\rm B\kern-.05em{\sc i\kern-.025em b}\kern-.08em
    T\kern-.1667em\lower.7ex\hbox{E}\kern-.125emX}}
\usepackage{balance}

\begin{document}

\maketitle

\bibliographystyle{IEEEtran}
\input{sections/appendix}
\bibliography{egbib}

\end{document}
